# Supplementary material for: IF-MDM: Implicit Face Motion Diffusion Model for High-Fidelity Realtime Talking Head Generation
Source: arXiv:2412.04000 source file (2024-12-10)
Supplement: Supplementary file 1 [file appendix.tex]

\counterwithin{figure}{section}

\appendix
